# Supplementary material for: Multi-Modal Mutual Information Maximization: A Novel Approach for Unsupervised Deep Cross-Modal Hashing
Source: arXiv:2112.06489 source file (2021-12-13)
Supplement: Supplementary file 1 [file appendix.tex]

\begin{table*}[t]
\begin{appendices}
%\clearpage
% \onecolumn

\section{More detail derivation of Equation \eqref{eq:private_info_upper_bound}}
\label{appendix:detail_upper_bound}

\begin{equation}
\tag{\ref{eq:private_info_upper_bound}}
\begin{split}
% \label{eq:private_info_upper_bound}
I(\bxi; \bhi|\bxt)&= \bbE_{\bsxi;\bsxt\sim p(\bxi,\bxt)}\bbE_{\bsh\sim P_{\theta_i} (\bhi|\bxi)} \left[\log \frac{p(\bxi = \bsxi,\bhi = \bsh|\bxt = \bsxt)}{p(\bxi = \bsxi|\bxt = \bsxt) P_{\theta_i} (\bhi = \bsh|\bxt = \bsxt)}\right] \\
&= \bbE_{\bsxi;\bsxt\sim p(\bxi,\bxt)}\bbE_{\bsh\sim P_{\theta_i} (\bhi|\bxi)} \left[\log \frac{p(\bxi = \bsxi|\bxt = \bsxt) P_{\theta_i}(\bhi = \bsh|\bxi = \bsxi,\bxt = \bsxt)}{p(\bxi = \bsxi|\bxt = \bsxt) P_{\theta_i} (\bhi = \bsh|\bxt = \bsxt)}\right]  \\
&= \bbE_{\bsxi;\bsxt\sim p(\bxi,\bxt)}\bbE_{\bsh\sim P_{\theta_i} (\bhi|\bxi)} \left[\log \frac{P_{\theta_i} (\bhi = \bsh|\bxi = \bsxi)}{P_{\theta_i} (\bhi = \bsh|\bxt = \bsxt)}\right]  \\
&= \bbE_{\bsxi;\bsxt\sim p(\bxi,\bxt)}\bbE_{\bsh\sim P_{\theta_i} (\bhi|\bxi)} \left[\log \frac{P_{\theta_i} (\bhi = \bsh|\bxi = \bsxi)}{P_{\theta_t} (\bht = \bsh|\bxt = \bsxt)}\right] \\
&\qquad\qquad\qquad\qquad+ \bbE_{\bsxi;\bsxt\sim p(\bxi,\bxt)}\bbE_{\bsh\sim P_{\theta_i} (\bhi|\bxi)} \left[\log \frac{P_{\theta_t} (\bht = \bsh|\bxt = \bsxt)}{P_{\theta_i} (\bhi = \bsh|\bxt = \bsxt)}\right]  \\
&= \DKL\left[P_{\theta_i} (\bhi|\bxi)||P_{\theta_t} (\bht|\bxt)\right] - \DKL\left[P_{\theta_i} (\bht|\bxi)||P_{\theta_t} (\bht|\bxt)\right] \\
&\le \DKL\left[P_{\theta_i} (\bhi|\bxi)||P_{\theta_t} (\bht|\bxt)\right].
\end{split}
\end{equation}
Note that since $\bhi$ is completely determined by $\bxi$, $H(\bhi|\bxi)=0$.
% Note that, since $H(\bhi|\bxi)=0$; 
Consequently,
$\bhi$ and $\bxt$ are conditionally independent given $\bxi$, i.e.,
\begin{equation}
P_{\theta_i}(\bhi = \bsh|\bxi = \bsxi,\bxt = \bsxt)=P_{\theta_i}(\bhi = \bsh|\bxi = \bsxi)   
\vspace{-1em}
\end{equation}

% \end{table*}

% \begin{table}[]
%     \centering
%     \begin{tabular}{c|c}
%          &  \\
%          & 
%     \end{tabular}
%     \caption{Caption}
%     \label{tab:my_label}
% \end{table}

% \begin{equation}
%     \bsxi,\bsxt\sim p(\bxi, \bxt)
% \end{equation}
% \begin{equation}
%     \bshi\sim P(\bhi|\bxi=\bsxi)
% \end{equation}
% \begin{equation}
%     \bsht\sim P(\bht|\bxt=\bsxt)
% \end{equation}

% \begin{equation}
%     p(\bhi,\bht) = p(\bxi, \bxt)P(\bhi|\bxi)P(\bht|\bxt)
% \end{equation}
% \begin{equation}
%     p(\bhi) = p(\bxi)P(\bhi|\bxi)
% \end{equation}
% \begin{equation}
%     p(\bht) = p(\bxt)P(\bht|\bxt)
% \end{equation}
\end{appendices}
\end{table*}
